# Supplementary material for: Correlation-Attention Masked Temporal Transformer for User Identity Linkage Using Heterogeneous Mobility Data
Source: arXiv:2504.01979 source file (2025-03-28)
Supplement: Supplementary file 1 [file 8supplement.tex]

\section{Supplementary Material }
\begin{table}[h!]
\centering
\begin{tabular}{c|c}
\hline
\textbf{Notation} & \textbf{Definition} \\ \hline
${\cal U}_A$   & user sets of platform A \\ 
${\cal U}_B$ & user sets of platform B \\
$u_i$ & a user \\
$t$   & the timestamp of the check-in \\ 
$p$ & a POI \\
${\cal T}_{u_i}$ & the check-in sequence of $u_i$ \\
$\cal P$ & the POI sets of $p$ \\
$T$ & the time slot sets of $t$ \\
$f_\theta(\cdot)$ & a mapping function of \model \\
${{\bf{E}}_p}$ & the embeddings of each $p$ \\
${{\bf{E}}_t}$ & the embeddings of each time slot of $t$ \\
$x$ & the joint embeddings of ${{\bf{E}}_p}$ and ${{\bf{E}}_t}$\\
${\bf{X}}$ & the embeddings of check-in sequences \\
$f_{st}(\cdot)$ & the spatial-temporal embedding layer \\
${\bf{z}}$ & the spatial-temporal embedding of $x$ \\
${\bf{Z}}$ & the spatial-temporal embeddings of ${\bf{z}}$ \\
${f_{\rm T}}(\cdot)$ & the temporal transformer encoder \\
${\bf{H}}$ & the spatio-temporal representation \\
${\bf{Q}}$ & the query vector of ${\bf{H}}$ \\
${\bf{K}}$ & the key vector of ${\bf{H}}$ \\
${\bf{V}}$ & the value vector of ${\bf{H}}$ \\
$H$ & number of heads for multi-head attention \\
$h$ & the $h$-th attention head \\
${\bf{Attn}}$ & the attention weight map \\
${f_{\rm M}}(\cdot)$ & the masked transformer encoder \\
${{\bf{I}}}$ & the index vector of attention weight map \\
${\bf{H}}^m$ & the representation of masked transformer \\
${{\bf{M}}_{mask}}$ & the mask matrix \\
\hline
\end{tabular}
\caption{Summary of key notations.}
\label{tab:notations}
\end{table}
\begin{table}[h!]
\centering
\begin{tabular}{c|cc}
\hline
\textbf{Hyperparameters} & $f_{\rm M}$ & $f_{\rm T}$ \\ \hline
POI embedding dimension         & 64 & 64 \\ 
time embedding dimension        & 16 & 16 \\ 
check-in embedding dimension    & 64 & 64 \\ 
Layers                          & 4 & 4 \\ 
FFN inner hidden size           & 128 & 128 \\ 
Attention heads                 & 8 & 8 \\ 
Attention head size             & 8  & 8 \\ 
\midrule
Training epochs                 & \multicolumn{2}{c}{50} \\ 
Batch size                      & \multicolumn{2}{c}{32} \\ 
Initial learning rate           & \multicolumn{2}{c}{1e-3} \\ 
Learning rate schedule          & \multicolumn{2}{c}{multiplicative (5, 0.9)} \\ 
Dropout                         & \multicolumn{2}{c}{0.1} \\ 
\midrule
mask ratio                       & \multicolumn{2}{c}{0.15} \\ 
\hline
\end{tabular}
\caption{Hyperparameters for $f_{\rm M}$ and $f_{\rm T}$ models.}
\label{tab:parameters}
\end{table}

\subsection{Notations}
Key notations used in the paper and their definitions are summarized in Table~\ref{tab:notations}

\subsection{Detailed Dataset Description}
For two publicly available cross-platform datasets, we applied the following processing steps:
\begin{itemize}
\item \textbf{XSiteTraj}: This dataset offers extensive spatial and temporal coverage, with over 27,000 users and more than one million check-ins collected from Facebook, Foursquare, and Twitter worldwide. It identifies the same users across different social platforms, and each check-in includes a timestamp, Point of Interest (POI), and POI coordinates. Due to the heterogeneity of data from different platforms and time zone differences, we used the H3 hierarchical geo-spatial indexing system to standardize check-in granularity and convert all timestamps to Universal Time Coordinated (UTC). We then arranged all check-ins for each user into a single, complete sequence based on UTC order. To facilitate training, we remove sequences longer than 400, 200, and 200 from the Twitter, Foursquare, and Facebook datasets, respectively, as these represent a small proportion of the data(5.20\%, 0.28\%, 0.17\%).

\item \textbf{ISP-Weibo}: DPLink and DPLink-SM utilize two real-world cross-domain mobile datasets. The ISP dataset includes mobile network records from one of China's largest ISPs and location-based social network data from Weibo. The ISP data covers Shanghai from April 19 to April 26, 2016, capturing location records generated at the cell tower level when users access the cellular network via mobile devices. The Weibo dataset is derived from the ISP dataset, with Weibo session data collected from the same time window by ISP collaborators, with Weibo's permission. We used the H3 hierarchical geo-spatial indexing system to standardize check-in granularity while preserving the original time granularity of the dataset. In the Weibo dataset, all check-ins for each user are merged into a single sequence based on timestamp order. In the ISP dataset, check-ins for each user are divided into multiple sequences based on daily time cycles (24 hours). Therefore, each user in the Weibo dataset has a single check-in sequence, while in the ISP dataset, each user has multiple sequences. We remove sequences shorter than 3 from the ISP and Weibo datasets, as they account for a small percentage of the data (3.53\%, 0.13\%).
\end{itemize}

\subsection{Detailed Experimental Settings}
The parameter settings for the experiment are shown in the table~\ref{tab:parameters}. All experiments are conducted on a machine with Intel (R) Xeon(R) Silver 4214 CPU @ 2.20GHz 12 cores CPU and NVIDIA NVIDIA GeForce RTX 3090 (24GB Memory) GPU.

To simulate real-world scenarios in the UIL task, specifically addressing class imbalance, we assigned positive and negative sample pairs before inputting them into the model. In the XSiteTraj dataset, positive samples were formed by pairing unique check-in sequences of the same user across two platforms, labeled as 1, while negative samples paired different users' sequences, labeled as 0, with a final ratio of 1:6 between positive and negative samples. Finally, once all positive and negative sample pairs for the same users in the dataset were assigned, we fed the data into the model. In the ISP-weibo dataset, positive samples were created by pairing the unique check-in sequence of the same user in Weibo with multiple sequences from the ISP dataset, while negative samples were formed by pairing sequences from different users across the two platforms, achieving a ratio of 1:2 between positive and negative samples. Finally, once all positive and negative sample pairs for the same users in the dataset were assigned, we fed the data into the model. To prevent data leakage in both XSiteTraj and ISP-weibo, we independently and randomly sampled the training, validation, and test sets for each platform. 

\subsection{Time Complexity Analysis}
We will analyze the operations of each main component step by step. The time complexity of the transformer is primarily determined by matrix multiplication, the computation of the attention mechanism, and the embedding operations. Assuming a batch size of $B$, the sequence lengths of both platforms are standardized to $S$, embedding dimension of $E$, number of attention heads $H$, and the dimension of the matrix after linear transformation is $d_k$, where $d_k = E/H$. The temporal transformer encoder has $L_t$ layers, the masked transformer encoder has $L_m$ layers, and the correlation attention block has $L_c$ layers.
\begin{itemize}
\item \textbf{Spatial-Temporal Embedding Layer}
In the computation of spatio-temporal embeddings, the operations involved include position embedding, time embedding, positional encoding, concatenation, and linear transformation. Since the linear transformation involves matrix multiplication, it has the highest computational cost, resulting in higher complexity. We can estimate the time complexity of each module mentioned above $O(B \times S \times E)$, $O(B \times S \times (E/4))$, $O(B \times S \times E)$ and $O(B \times S \times {E^2})$. Finally, the overall time complexity can be approximated as $O(B \times S \times {E^2})$. This reflects the dominant cost of the linear transformation in the process.

\item \textbf{Temporal Transformer Encoder}
In the temporal transformer encoder, the main operations are attention calculation and the feedforward neural network. The time complexity of the attention calculation is $O(H \times {S^2} \times {d_k}) = O({S^2} \times E)$. The time complexity of the feed-forward neural network is $O(B \times S \times {E^2})$. Therefore, the overall time complexity of the temporal transformer encoder can be approximated as $O(L_t \times B \times ({S^2} \times E + S \times {E^2}))$. 

\item \textbf{Correlation Attention Block}
The main complexity of cross-attention arises from the calculation involving sequences from two different platforms. If we standardize the length of the two sequences to $S$, the time complexity can be approximated as $O({L_c} \times B \times S \times E)$.

\item \textbf{Masked Transformer Encoder}
In the masked transformer encoder, the complexity of generating the mask primarily depends on attention weight filtering and mask application. The time complexity of mask calculation is $O(B \times {S^2})$. During the top-K element selection, since for each batch and each sequence, $K$ elements are selected from $S$ elements, the complexity is $O(B \times S\log S)$. Finally, the complexity of applying the mask is $O(B \times S \times {E})$. Therefore, the overall time complexity is $O(B \times {S^2} + B \times S\log S + B \times S \times E)$. We take the dominant complexity as the main focus and simplify it as $O(B \times {S^2})$. In the transformer computations, the complexity is similar to that of the temporal transformer encoder. Thus, the total time complexity can be expressed as $O(B \times {S^2} + {L_m} \times B \times ({S^2} \times E + S \times {E^2}))$. 
\end{itemize}

In summary, the total time complexity of the model is $O(B \times S \times {E^2} + {L_t} \times B \times ({S^2} \times E + S \times {E^2}) + {L_c} \times B \times S \times E + B \times {S^2} + {L_m} \times B \times ({S^2} \times E + S \times {E^2}))$.

By retaining the highest-order dominant term, the time complexity can be approximated as $O(({L_t} + {L_m}) \times B \times {S^2} \times E)$. This expression indicates that when the sequence length $S$ and embedding dimension $E$ are large, the time complexity is primarily influenced by the quadratic relationship with the sequence length and the linear relationship with the embedding dimension.
